# Supplementary material for: Accelerating Molecular Dynamics Simulations with Foundation Neural Network Models using Multiple Time-Step and Distillation
Source: arXiv:2510.06562 ancillary file (2026-01-09)
Supplement: Supplementary file 1 [file SI-MTS-v2.pdf]

# Supporting Information for: Accelerating Molecular Dynamics Simulations with Foundation Neural Network Models using Multiple Time-Step and Distillation

Côme Cattin,<sup>†</sup> Thomas Plé,<sup>\*,†</sup> Olivier Adjoua,<sup>†</sup> Nicolai Gouraud,<sup>‡</sup> Louis  
Lagardère,<sup>†</sup> and Jean-Philip Piquemal<sup>\*,†</sup>

<sup>†</sup>*Sorbonne Université, Laboratoire de Chimie Théorique, UMR 7616 CNRS, 75005 Paris,  
France*

<sup>‡</sup>*Qubit Pharmaceuticals, Advanced Research Department, 75014 Paris, France*

E-mail: thomas.ple@sorbonne-universite.fr; jean-philip.piquemal@sorbonne-universite.fr

## Model and training details

**Model architecture** For both the reference and distilled models, we initialize the atomic descriptors from an encoding of the electronic structure of isolated atoms and include charge information via a non-local total charge embedding as described in ref.<sup>?</sup> The dimension of the atomic embedding is 176 for the large model and 96 for the small model. We then incorporate local geometric information via an equivariant message-passing neural network. For the large model, we perform two message-passing iterations with an interaction cutoff of 3.5Å for the first one and 7.5Å for the second one. The small model only performs one message-passing iteration with an interaction cutoff of 3.5Å. It is thus much more short-sighted than the large model, biasing it to focus on the shorter-range interactions responsible for the high-

frequency vibrations. Atomic energies are then obtained from mixture-of-experts multi-layer perceptrons where routing is performed by blocks in the periodic table (see Supplementary Information of ref.<sup>7</sup> for details).

**Model training** The loss function for the distillation includes atomic energies from the FeNNix-Bio1(M) energy decomposition (weight 100), total energies (weight 20), and forces (weight 1000). We used an Adabelief optimizer<sup>7</sup> with an initial learning rate of  $2 \times 10^{-4}$ , and a final learning rate of  $1 \times 10^{-7}$ , combined with cosine one-cycle learning rate schedule.

For bulk water and solvated molecules, reference datasets were generated by running a 200 ps NVT molecular dynamics simulation for each system using the reference model. The conformations were sampled every 0.2 ps, resulting in 1000 frames per system. The resulting dataset is then shuffled and split into 800 training frames and 200 validation frames.

For proteins and, more generally, for large systems, a fragmentation strategy was employed to reduce the computational burden and memory requirements of training the model. In this approach, random fragments are extracted from the protein by first selecting central atoms at random (100 centers for water and ions, and 500 centers for proteins). Hydrogen atoms were excluded from being chosen as centers. Around each selected atom, a spherical environment with a radius of 5 Å was constructed and the cut covalent bonds were saturated with hydrogen atoms. For training models on the phenol-lysozyme complex, 50 frames from the first 500 ps of simulation, were used, resulting in a dataset of 30,000 fragments.
